# Supplementary material for: Distribution Regression with Sample Selection, with an Application to Wage Decompositions in the UK
Source: arXiv:1811.11603 source file (2023-12-18)

# Estimates of Parameters, Male in 1978 ~ 2013

**numch1**

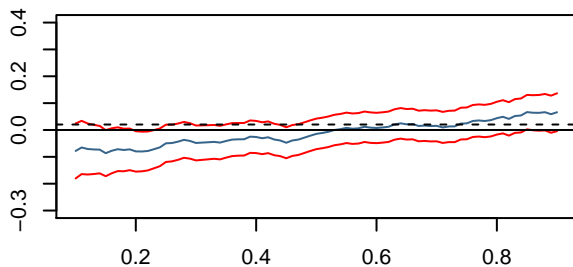

**numch2**

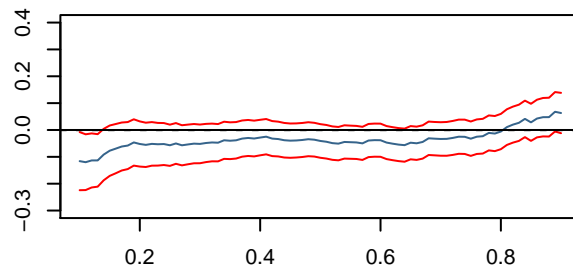

**numch34**

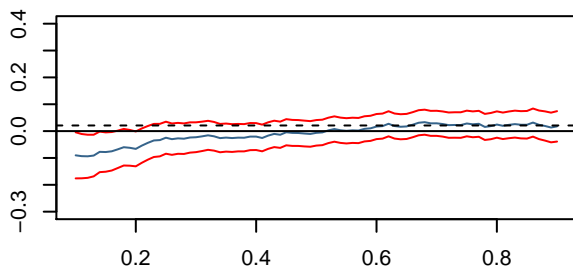

**numch510**

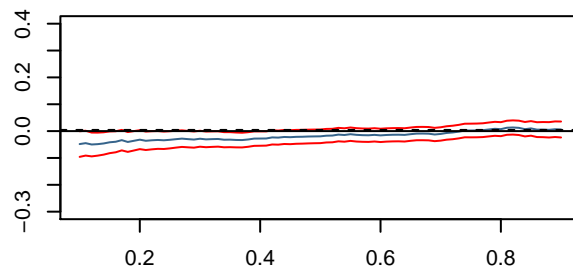

**numch1116**

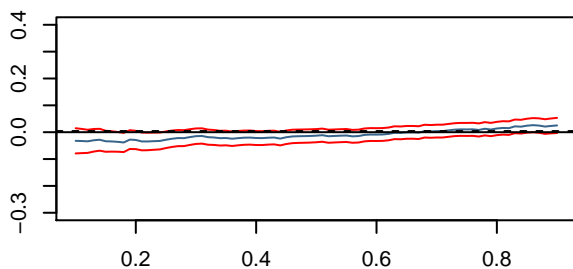

**numch1718**

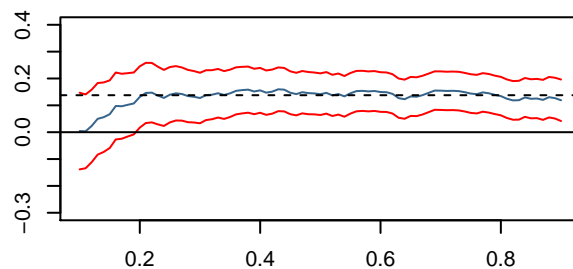

Estimates of Unobserved Selection, Male in 1978 ~ 2013

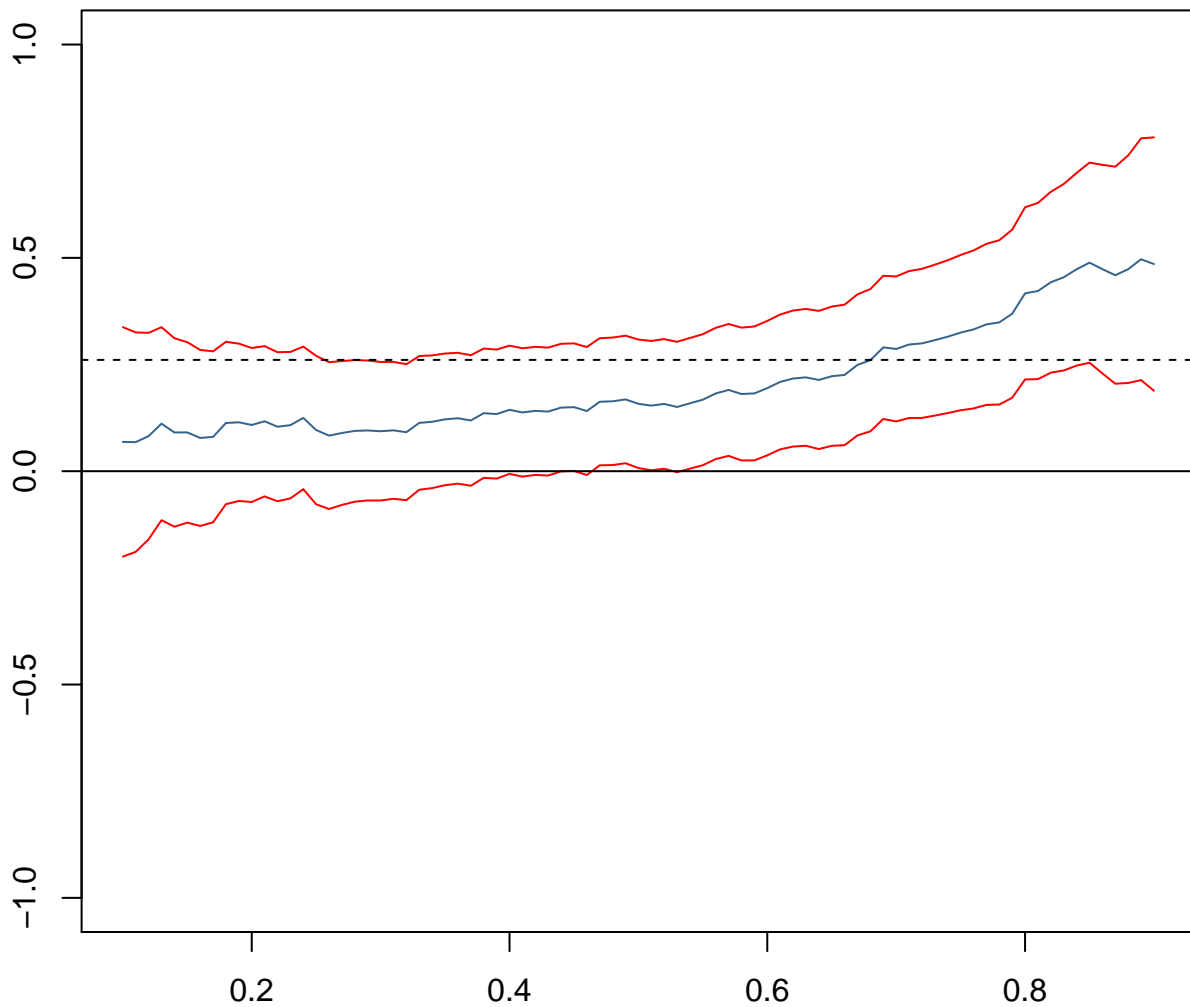

# Estimates of Parameters, Female in 1978 ~ 2013

**numch1**

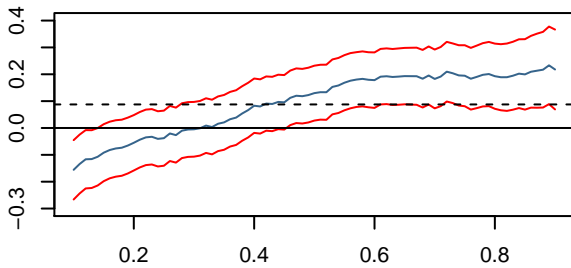

**numch2**

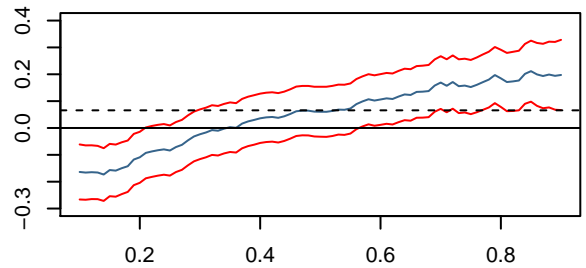

**numch34**

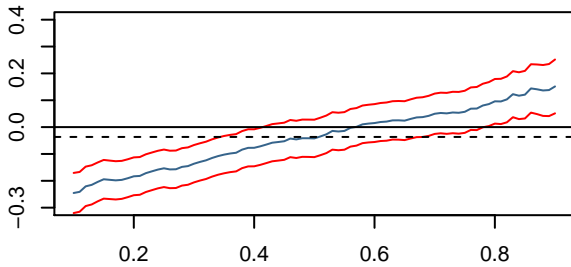

**numch510**

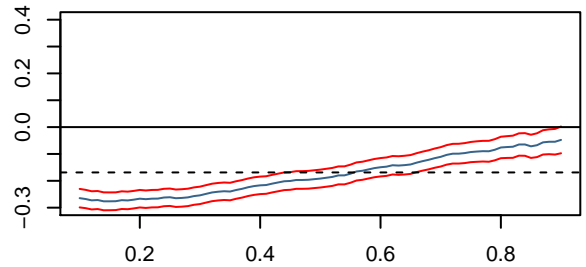

**numch1116**

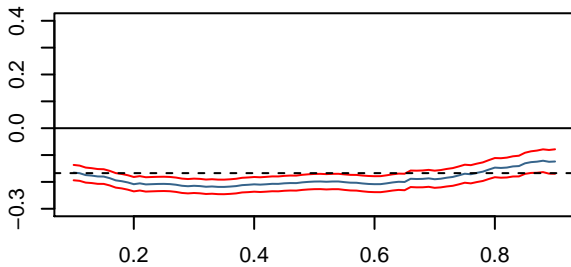

**numch1718**

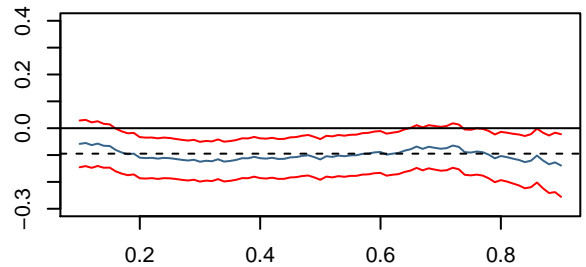

Estimates of Unobserved Selection, Female in 1978 ~ 2013

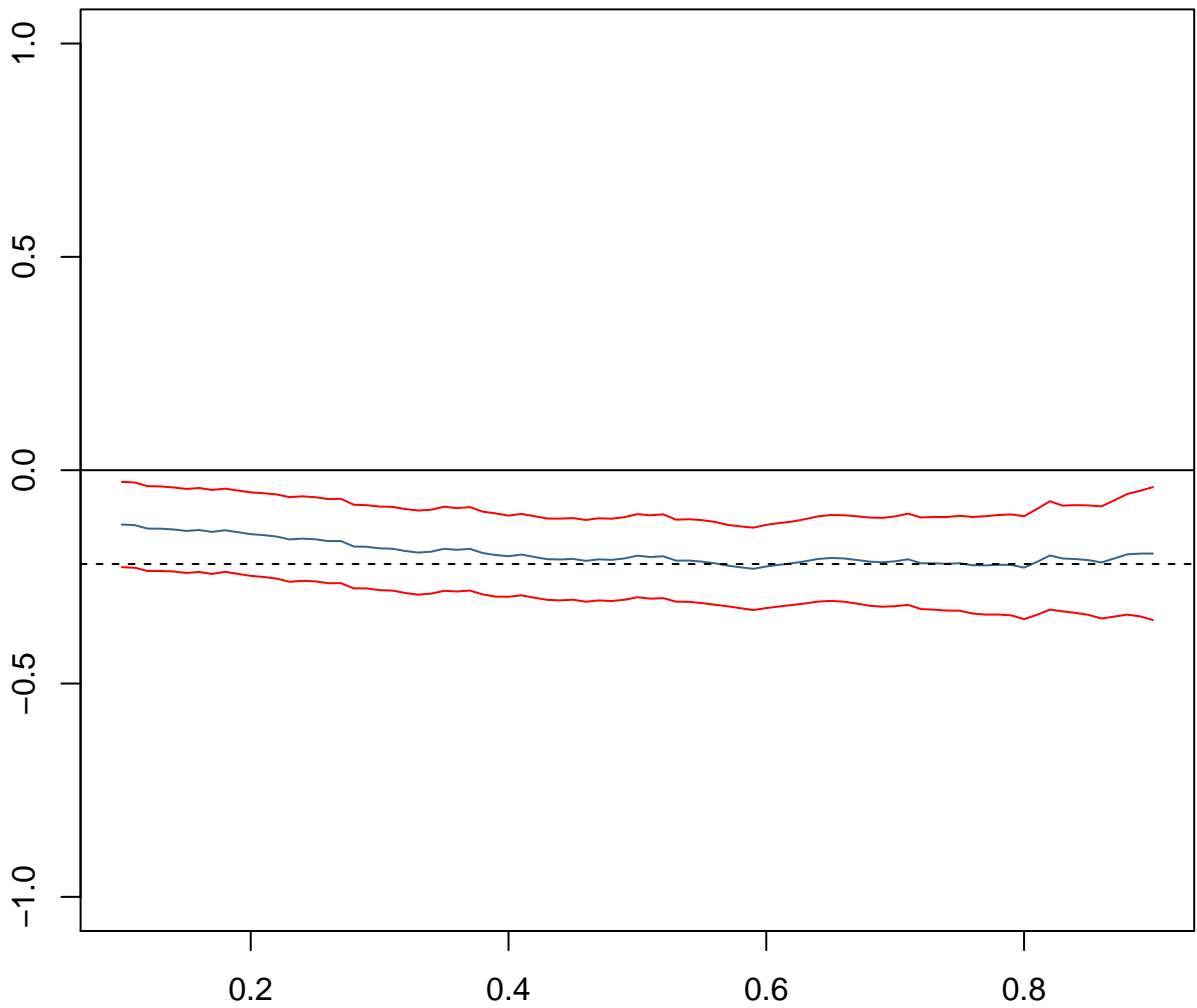

Comparison of Unobserved Selection, 1978 ~ 2013 (male vs. female)

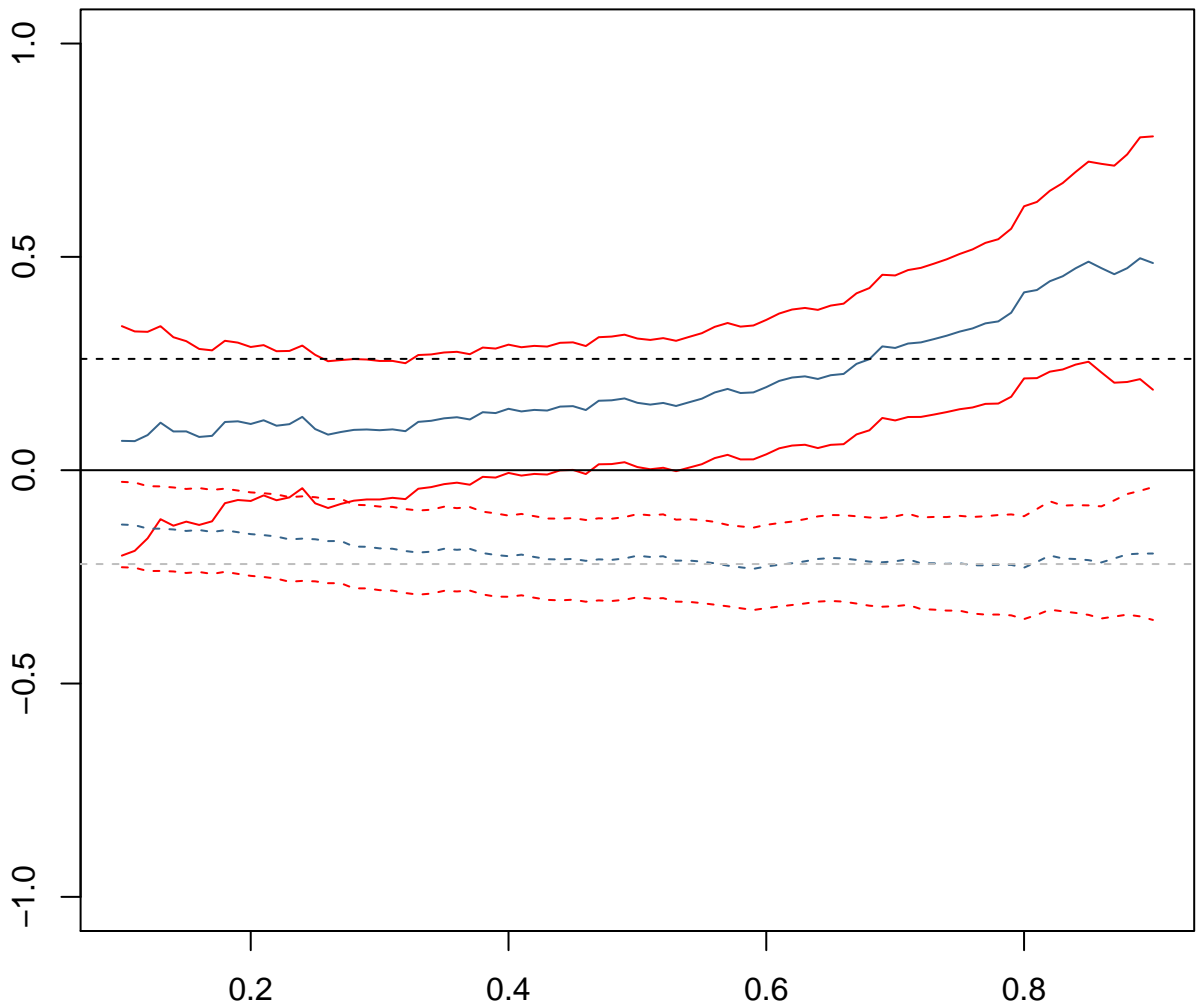

Supplement: Supplementary file 1 [file Estimates_suppl_11378_500.pdf]
